# Supplementary material for: Early Risk Prediction of Pediatric Cardiac Arrest from Electronic Health Records via Multimodal Fused Transformer
Source: arXiv:2502.07158 source file (2025-05-20)
Supplement: Supplementary file 1 [file appendix.tex]

\clearpage
\begin{appendices}
\section{Early Explorations On Feature Selection}
\subsection{LLM-fprune: LLM-based feature selection method}
We prompt the . 

\begin{table}[ht!]
    \caption{Toy case of LLM-fprune}
    \label{tab:toy_case_fprune}
    \centering
    \begin{tabular}{p{0.10\linewidth} | p{0.85\linewidth}}
    \toprule
    User\textless:& I am trying to decide which feature can be used to predict pediatric patient's cardiac arrest. Can you help me by answering "yes" if the feature should be pruned, "no" vice verse. \newline Shall I prune \textbf{"heart rate"} for cardiac arrest prediction? \\ \hline
    LLM\textgreater:& \textbf{No}, you should not prune "heart rate" for cardiac arrest prediction. Heart rate is a crucial indicator of cardiac function and can be a significant predictor of cardiac arrest.\\
    \midrule
    User\textless:& Shall I prune \textbf{"bed position"} for cardiac arrest prediction?\\ \hline
    LLM\textgreater:& \textbf{Yes}, you can prune "bed position" for cardiac arrest prediction. Bed position is unlikely to be a direct predictor of cardiac arrest in pediatric patients.\\
    \bottomrule
    \end{tabular}
\end{table}

\subsection{Feature Selection Experiments}
To disentangle the impact of imbalanced case and control samples, we evaluate the feature selection methods on a curated balanced version of dataset. We will include hand-crafted feature selection method, data-driven feature selection method and our own LLM-based feature selection method.
\begin{itemize}
    \item Emb-score: .
    \item LLM-fprune: our feature selection method that explicitly output whether one specific feature should be pruned for the task of interest.
\end{itemize}

\begin{table}[ht!]
\centering
\caption{Feature selection experimental results.}
\label{tab:feat_sele}
\begin{tabular}{c|ccc|ccc}
\toprule
\multirow{2}{*}{FS Method} & \multicolumn{3}{c|}{PIC} & \multicolumn{3}{|c}{CHOA-CICU}\\ 
& Bal\_Acc & F1 & AUROC & Bal\_Acc & F1 & AUROC\\
\midrule
& \multicolumn{6}{c}{TabNeuralNet}\\
All & \\
Coverage &  \\
Lasso & \\
MI & \\
Emb-score & \\
LLM-fprune & \\
\hline
& \multicolumn{6}{c}{LightGBM}\\
&  \\
\hline
& \multicolumn{6}{c}{XGBoost}\\
&  \\
\bottomrule
\end{tabular}
\end{table}

\subsection{Training Sample Selection Experiments}

\end{appendices}
